# Supplementary material for: Adversarial Attack on Network Embeddings via Supervised Network Poisoning
Source: arXiv:2102.07164 source file (2021-02-14)
Supplement: Supplementary file 1 [file Appendix_Vals.pdf]

| Cora Combined Edges | | | | | | | | |
|---|---|---|---|---|---|---|---|---|
| | SkipGram Deepwalk | | SVD Deepwalk | | LINE | | Node2Vec | |
| | F1 Micro | F1 Macro | F1 Micro | F1 Macro | F1 Micro | F1 Macro | F1 Micro | F1 Macro |
| cln, | 0.81 | 0.78 | 0.82 | 0.80 | 0.74 | 0.70 | 0.76 | 0.70 |
| rnd, | 0.76 | 0.73 | 0.78 | 0.76 | 0.73 | 0.69 | 0.71 | 0.65 |
| deg, | 0.74 | 0.71 | 0.77 | 0.75 | 0.74 | 0.70 | 0.65 | 0.58 |
| our, | 0.68 | 0.65 | 0.72 | 0.70 | 0.74 | 0.71 | 0.58 | 0.50 |
| ori, | 0.72 | 0.68 | 0.76 | 0.74 | 0.73 | 0.70 | 0.67 | 0.60 |

| Cora Edge Addition | | | | | | | | |
|---|---|---|---|---|---|---|---|---|
| | SkipGram Deepwalk | | SVD Deepwalk | | LINE | | Node2Vec | |
| | F1 Micro | F1 Macro | F1 Micro | F1 Macro | F1 Micro | F1 Macro | F1 Micro | F1 Macro |
| cln, | 0.81 | 0.78 | 0.82 | 0.80 | 0.75 | 0.71 | 0.77 | 0.72 |
| rnd, | 0.74 | 0.70 | 0.76 | 0.74 | 0.75 | 0.71 | 0.70 | 0.64 |
| deg, | 0.74 | 0.71 | 0.77 | 0.75 | 0.75 | 0.71 | 0.70 | 0.64 |
| our, | 0.68 | 0.65 | 0.72 | 0.70 | 0.75 | 0.72 | 0.65 | 0.59 |
| ori, | 0.79 | 0.76 | 0.81 | 0.78 | 0.75 | 0.72 | 0.75 | 0.69 |

| Cora Edge Removal | | | | | | | | |
|---|---|---|---|---|---|---|---|---|
| | SkipGram Deepwalk | | SVD Deepwalk | | LINE | | Node2Vec | |
| | F1 Micro | F1 Macro | F1 Micro | F1 Macro | F1 Micro | F1 Macro | F1 Micro | F1 Macro |
| cln, | 0.80 | 0.77 | 0.82 | 0.80 | 0.73 | 0.69 | 0.79 | 0.75 |
| rnd, | 0.80 | 0.77 | 0.81 | 0.79 | 0.73 | 0.68 | 0.77 | 0.72 |
| deg, | 0.77 | 0.73 | 0.79 | 0.76 | 0.74 | 0.70 | 0.70 | 0.62 |
| our, | 0.75 | 0.71 | 0.77 | 0.74 | 0.73 | 0.69 | 0.71 | 0.64 |
| ori, | 0.73 | 0.69 | 0.76 | 0.74 | 0.73 | 0.69 | 0.68 | 0.62 |

| FFire Combined Edges | | | | | | | | |
|---|---|---|---|---|---|---|---|---|
| | SkipGram Deepwalk | | SVD Deepwalk | | LINE | | Node2Vec | |
| | F1 Micro | F1 Macro | F1 Micro | F1 Macro | F1 Micro | F1 Macro | F1 Micro | F1 Macro |
| cln, | 0.67 | 0.28 | 0.76 | 0.43 | 0.68 | 0.32 | 0.49 | 0.13 |
| rnd, | 0.55 | 0.20 | 0.59 | 0.27 | 0.67 | 0.31 | 0.38 | 0.08 |
| deg, | 0.55 | 0.19 | 0.59 | 0.26 | 0.67 | 0.31 | 0.32 | 0.06 |
| our, | 0.53 | 0.19 | 0.57 | 0.25 | 0.68 | 0.31 | 0.31 | 0.06 |
| ori, | 0.55 | 0.21 | 0.63 | 0.31 | 0.66 | 0.30 | 0.40 | 0.08 |

| FFire Edge Addition | | | | | | | | |
|---|---|---|---|---|---|---|---|---|
| | SkipGram Deepwalk | | SVD Deepwalk | | LINE | | Node2Vec | |
| | F1 Micro | F1 Macro | F1 Micro | F1 Macro | F1 Micro | F1 Macro | F1 Micro | F1 Macro |
| cln, | 0.68 | 0.29 | 0.76 | 0.43 | 0.67 | 0.31 | 0.47 | 0.11 |
| rnd, | 0.52 | 0.19 | 0.57 | 0.24 | 0.68 | 0.31 | 0.36 | 0.07 |
| deg, | 0.55 | 0.20 | 0.59 | 0.27 | 0.66 | 0.30 | 0.30 | 0.06 |
| our, | 0.54 | 0.19 | 0.57 | 0.25 | 0.67 | 0.31 | 0.36 | 0.07 |
| ori, | 0.61 | 0.25 | 0.70 | 0.39 | 0.68 | 0.31 | 0.41 | 0.09 |

| FFire Edge Removal | | | | | | | | |
|---|---|---|---|---|---|---|---|---|
| | SkipGram Deepwalk | | SVD Deepwalk | | LINE | | Node2Vec | |
| | F1 Micro | F1 Macro | F1 Micro | F1 Macro | F1 Micro | F1 Macro | F1 Micro | F1 Macro |
| cln, | 0.68 | 0.28 | 0.76 | 0.43 | 0.66 | 0.30 | 0.47 | 0.11 |
| rnd, | 0.65 | 0.28 | 0.73 | 0.40 | 0.68 | 0.32 | 0.42 | 0.09 |
| deg, | 0.59 | 0.22 | 0.64 | 0.29 | 0.68 | 0.31 | 0.43 | 0.10 |
| our, | 0.58 | 0.24 | 0.62 | 0.31 | 0.67 | 0.30 | 0.42 | 0.10 |
| ori, | 0.55 | 0.19 | 0.63 | 0.31 | 0.67 | 0.31 | 0.37 | 0.07 |

| PolBlogs Combined Edges | | | | | | | | |
|---|---|---|---|---|---|---|---|---|
| | SkipGram Deepwalk | | SVD Deepwalk | | LINE | | Node2Vec | |
| | F1 Micro | F1 Macro | F1 Micro | F1 Macro | F1 Micro | F1 Macro | F1 Micro | F1 Macro |
| cln, | 0.95 | 0.95 | 0.95 | 0.95 | 0.94 | 0.94 | 0.95 | 0.95 |
| rnd, | 0.95 | 0.95 | 0.95 | 0.95 | 0.94 | 0.94 | 0.94 | 0.94 |
| deg, | 0.93 | 0.93 | 0.89 | 0.89 | 0.94 | 0.94 | 0.94 | 0.94 |
| our, | 0.81 | 0.81 | 0.83 | 0.83 | 0.94 | 0.94 | 0.84 | 0.84 |
| ori, | 0.95 | 0.95 | 0.94 | 0.94 | 0.94 | 0.94 | 0.95 | 0.95 |

| PolBlogs Edge Addition | | | | | | | | |
|---|---|---|---|---|---|---|---|---|
| | SkipGram Deepwalk | | SVD Deepwalk | | LINE | | Node2Vec | |
| | F1 Micro | F1 Macro | F1 Micro | F1 Macro | F1 Micro | F1 Macro | F1 Micro | F1 Macro |
| cln, | 0.95 | 0.95 | 0.95 | 0.95 | 0.94 | 0.94 | 0.95 | 0.95 |
| rnd, | 0.93 | 0.93 | 0.94 | 0.94 | 0.94 | 0.94 | 0.94 | 0.94 |
| deg, | 0.93 | 0.93 | 0.89 | 0.89 | 0.94 | 0.94 | 0.93 | 0.93 |
| our, | 0.81 | 0.81 | 0.83 | 0.83 | 0.94 | 0.94 | 0.82 | 0.82 |
| ori, | 0.95 | 0.95 | 0.95 | 0.95 | 0.94 | 0.94 | 0.95 | 0.95 |

| PolBlogs Edge Removal | | | | | | | | |
|---|---|---|---|---|---|---|---|---|
| | SkipGram Deepwalk | | SVD Deepwalk | | LINE | | Node2Vec | |
| | F1 Micro | F1 Macro | F1 Micro | F1 Macro | F1 Micro | F1 Macro | F1 Micro | F1 Macro |
| cln, | 0.95 | 0.95 | 0.95 | 0.95 | 0.93 | 0.93 | 0.95 | 0.95 |
| rnd, | 0.95 | 0.95 | 0.95 | 0.95 | 0.94 | 0.94 | 0.95 | 0.95 |
| deg, | 0.95 | 0.95 | 0.95 | 0.95 | 0.94 | 0.94 | 0.95 | 0.95 |
| our, | 0.89 | 0.89 | 0.90 | 0.90 | 0.94 | 0.94 | 0.89 | 0.89 |
| ori, | 0.95 | 0.95 | 0.95 | 0.95 | 0.93 | 0.93 | 0.94 | 0.94 |

| CiteSeer Combined Edges | | | | | | | | |
|---|---|---|---|---|---|---|---|---|
| | SkipGram Deepwalk | | SVD Deepwalk | | LINE | | Node2Vec | |
| | F1 Micro | F1 Macro | F1 Micro | F1 Macro | F1 Micro | F1 Macro | F1 Micro | F1 Macro |
| cln, | 0.84 | 0.43 | 0.85 | 0.44 | 0.82 | 0.42 | 0.79 | 0.40 |
| rnd, | 0.74 | 0.37 | 0.76 | 0.38 | 0.83 | 0.42 | 0.70 | 0.33 |
| deg, | 0.78 | 0.39 | 0.78 | 0.39 | 0.82 | 0.42 | 0.70 | 0.32 |
| our, | 0.66 | 0.32 | 0.69 | 0.34 | 0.83 | 0.42 | 0.61 | 0.26 |
| ori, | 0.67 | 0.34 | 0.71 | 0.35 | 0.81 | 0.42 | 0.62 | 0.28 |

| CiteSeer Edge Addition | | | | | | | | |
|---|---|---|---|---|---|---|---|---|
| | SkipGram Deepwalk | | SVD Deepwalk | | LINE | | Node2Vec | |
| | F1 Micro | F1 Macro | F1 Micro | F1 Macro | F1 Micro | F1 Macro | F1 Micro | F1 Macro |
| cln, | 0.84 | 0.43 | 0.85 | 0.44 | 0.82 | 0.42 | 0.77 | 0.38 |
| rnd, | 0.75 | 0.37 | 0.77 | 0.39 | 0.83 | 0.43 | 0.71 | 0.34 |
| deg, | 0.78 | 0.39 | 0.78 | 0.40 | 0.83 | 0.43 | 0.71 | 0.32 |
| our, | 0.66 | 0.32 | 0.69 | 0.34 | 0.82 | 0.42 | 0.62 | 0.26 |
| ori, | 0.78 | 0.40 | 0.81 | 0.41 | 0.83 | 0.43 | 0.69 | 0.30 |

| CiteSeer Edge Removal | | | | | | | | |
|---|---|---|---|---|---|---|---|---|
| | SkipGram Deepwalk | | SVD Deepwalk | | LINE | | Node2Vec | |
| | F1 Micro | F1 Macro | F1 Micro | F1 Macro | F1 Micro | F1 Macro | F1 Micro | F1 Macro |
| cln, | 0.84 | 0.43 | 0.85 | 0.44 | 0.83 | 0.43 | 0.76 | 0.37 |
| rnd, | 0.73 | 0.36 | 0.75 | 0.38 | 0.82 | 0.42 | 0.70 | 0.34 |
| deg, | 0.73 | 0.37 | 0.73 | 0.37 | 0.83 | 0.42 | 0.66 | 0.32 |
| our, | 0.65 | 0.33 | 0.70 | 0.34 | 0.82 | 0.42 | 0.58 | 0.26 |
| ori, | 0.69 | 0.34 | 0.70 | 0.34 | 0.83 | 0.42 | 0.64 | 0.29 |

| LFR Combined Edges + DeepWalk Skipgram (Micro F1) | | | | | | | |
|---|---|---|---|---|---|---|---|
| mu= | 0.10 | 0.20 | 0.30 | 0.40 | 0.50 | 0.60 | 0.70 |
| cln, | 1.00 | 0.96 | 0.75 | 0.54 | 0.52 | 0.52 | 0.54 |
| rnd, | 1.00 | 0.96 | 0.73 | 0.53 | 0.52 | 0.51 | 0.53 |
| deg, | 1.00 | 0.96 | 0.75 | 0.53 | 0.52 | 0.52 | 0.53 |
| our, | 1.00 | 0.93 | 0.68 | 0.52 | 0.51 | 0.52 | 0.55 |
| ori, | 1.00 | 0.95 | 0.72 | 0.52 | 0.52 | 0.51 | 0.52 |

| LFR Addition Edges + DeepWalk Skipgram (Micro F1) | | | | | | | |
|---|---|---|---|---|---|---|---|
| mu= | 0.1 | 0.2 | 0.3 | 0.4 | 0.5 | 0.6 | 0.7 |
| cln, | 1.00 | 0.97 | 0.74 | 0.53 | 0.52 | 0.51 | 0.53 |
| rnd, | 1.00 | 0.97 | 0.73 | 0.54 | 0.52 | 0.50 | 0.53 |
| deg, | 1.00 | 0.96 | 0.74 | 0.53 | 0.52 | 0.51 | 0.52 |
| our, | 1.00 | 0.93 | 0.66 | 0.52 | 0.51 | 0.51 | 0.54 |
| ori, | 1.00 | 0.96 | 0.73 | 0.53 | 0.52 | 0.51 | 0.52 |

| LFR Removal Edges + DeepWalk Skipgram (Micro F1) | | | | | | | |
|---|---|---|---|---|---|---|---|
| mu= | 0.1 | 0.2 | 0.3 | 0.4 | 0.5 | 0.6 | 0.7 |
| cln, | 1.00 | 0.97 | 0.74 | 0.53 | 0.52 | 0.52 | 0.53 |
| rnd, | 1.00 | 0.96 | 0.72 | 0.53 | 0.52 | 0.52 | 0.52 |
| deg, | 1.00 | 0.96 | 0.75 | 0.53 | 0.51 | 0.51 | 0.52 |
| our, | 0.95 | 0.87 | 0.63 | 0.53 | 0.52 | 0.51 | 0.54 |
| ori, | 1.00 | 0.95 | 0.70 | 0.52 | 0.51 | 0.51 | 0.52 |

| Varying number of flips, PolBlogs + DeepWalk Skipgram (Micro F1) | | | | | | | |
|---|---|---|---|---|---|---|---|
| Percent Flips | 10% | 20% | 30% | 40% | 50% | 60% | 70% |
| Edges | 580 | 1160 | 1741 | 2321 | 2902 | 3482 | 4062 |
| cln, | 0.84 | 0.83 | 0.83 | 0.85 | 0.85 | 0.85 | 0.85 |
| rnd, | 0.78 | 0.73 | 0.69 | 0.68 | 0.65 | 0.57 | 0.56 |
| deg, | 0.81 | 0.76 | 0.73 | 0.72 | 0.70 | 0.66 | 0.63 |
| our, | 0.74 | 0.63 | 0.55 | 0.54 | 0.49 | 0.43 | 0.43 |
| ori, | 0.75 | 0.69 | 0.54 | 0.54 | 0.52 | 0.46 | 0.44 |
